# Supplementary material for: Deep Unsupervised Cardinality Estimation
Source: arXiv:1905.04278 source file (2019-11-21)
Supplement: Supplementary file 1 [file appendix.tex]

\begin{appendix}

\section{Proof of Theorem 1}
\label{appendix:proof}
% We now prove that progressive sampling is unbiased (\secref{sec:prog-sampling}).
\begin{proof}
The proof uses only basic probability rules.  For ease of exposition, we prove the 3-column case; the general N-column case
follows the exact structure.  Specifically, we need to show the expectation of
Equation~\ref{eq:three-col-progressive}, \begin{equation*}
\begin{aligned}
 &\expectation_{x_1^{(i)}, x_2^{(i)}} \left[ \phat(X_3 \in R_3 | x_1^{(i)}, x_2^{(i)})   \phat(X_2 \in R_2 | x_1^{(i)})  \phat(X_1 \in R_1) \right]
\end{aligned}
\end{equation*}
equals the desired density.  First, expanding the expectation over $x_1^{(i)}$ gives
\begin{equation*}
\begin{aligned}
  &\expectation_{x_2^{(i)}} \bigl[ \sum_{\substack{x_1=K \in R_1}}  \phat(x_1 = K | x_1 \in R_1)  \phat(X_3 \in R_3 | x_1 = K, x_2^{(i)})  \\
    & \qquad \qquad \qquad \phat(X_2 \in R_2 | x_1 = K)  \phat(X_1 \in R_1) \bigr]
\end{aligned}
\end{equation*}
Applying Bayes' rule to the new conditional term,
\begin{equation*}
\begin{aligned}
  &\expectation_{x_2^{(i)}} \bigl[\sum_{\substack{x_1=K \in R_1}}  \frac{\phat(x_1=K)}{\phat(X_1 \in R_1)}  \phat(X_3 \in R_3 | x_1 = K, x_2^{(i)})  \\
  &\qquad \qquad \qquad  \phat(X_2 \in R_2 | x_1 = K)  \phat(X_1 \in R_1) \bigr]
\end{aligned}
\end{equation*}
Similarly, we expand the expectation over $x_2^{(i)}$ and applying the same rule to get
\begin{equation*}
\begin{aligned}
  & \sum_{\substack{x_1=K \in R_1\\x_2=M \in R_2}} \bigl [ \frac{\phat(x_2 = M | x_1 = K)}{\phat(X_2 \in R_2 | x_1 = K)}\frac{\phat(x_1=K)}{\phat(X_1 \in R_1)} \\
  & \phat(X_3 \in R_3 | x_1=K, x_2=M) \phat(X_2 \in R_2 | x_1=K) \phat(X_1 \in R_1) \bigr]
\end{aligned}
\end{equation*}
Canceling terms, we obtain
\begin{equation*}
\begin{aligned}
 & \sum_{\substack{x_1=K \in R_1\\x_2=M \in R_2}} \bigl [\phat(X_3 \in R_3 | x_1=K, x_2=M) \phat(x_2 = M | x_1 = K)\\
&\qquad \qquad  \phat(x_1=K)  \bigr]
\end{aligned}
\end{equation*}
which is the density $\phat(X_1 \in R_1, X_2 \in R_2, X_3 \in R_3)$.
\end{proof}

\end{appendix}
